# Supplementary material for: Recovering high-quality FODs from a reduced number of diffusion-weighted images using a model-driven deep learning architecture
Source: arXiv:2307.15273 source file (2023-07-28)
Supplement: Supplementary file 1 [file 7.Supplementary.tex]

\begin{table*}
  \centering
  \resizebox{1\textwidth}{!}{
  \begin{tabular}{?c?l?llll?}
     \specialrule{1.25pt}{0pt}{0pt}
    \textbf{Metric} &\diagbox[innerwidth=1.5cm]{\textbf{Region}}{\textbf{Method}}& 
    \textbf{SDNet}&
    \textbf{SDNet\textsubscript{\boldmath$\kappa$} (p\textsubscript{SD})}&
    \textbf{FODNet (p\textsubscript{SD}, p\textsubscript{SD\boldmath${\kappa}$})} & \textbf{MSMT CSD (p\textsubscript{SD}, {p}\textsubscript{SD\boldmath$\kappa$})}\\
    \specialrule{1.1pt}{0pt}{0pt}
    \multirow{4}{*}{\textbf{\shortstack{SSE\\(\downarrow)}}} & 
    White Matter &
    \textbf{0.011$\pm$0.001} &
    0.012$\pm$0.001 ($<$\textbf{0.001})&
    0.013$\pm$0.001 ($<$\textbf{0.001}, 0.034)& 
    0.041$\pm$0.002 ($<$\textbf{0.001}, $<$\textbf{0.001}) \\
    &
    ROI-1-CC&
    \textbf{0.009$\pm$0.001}&
    0.010$\pm$0.001 ($<$\textbf{0.001}) &
    0.011$\pm$0.001 ($<$\textbf{0.001}, 0.295) &
    0.037$\pm$0.002 ($<$\textbf{0.001}, $<$\textbf{0.001}) \\
    
    &
    ROI-2-MCP &
     \textbf{0.020$\pm$0.001}&
    0.022$\pm$0.001 ($<$\textbf{0.001}) &
    0.022$\pm$0.001 (\textbf{0.001}, 0.175)&
    0.057$\pm$0.003 ($<$\textbf{0.001}, $<$\textbf{0.001})\\
    
    &
    ROI-3-SLF & 
    \textbf{0.012$\pm$0.001}&
    0.013$\pm$0.001 (\textbf{0.005})& 
    0.014$\pm$0.001 ($<$\textbf{0.001}, $<$\textbf{0.001})& 
    0.043$\pm$0.002 ($<$\textbf{0.001}, $<$\textbf{0.001})\\
    \specialrule{1.25pt}{0pt}{0pt}
    \multirow{4}{*}{\textbf{\shortstack{ACC\\(\uparrow)}}} &
    White Matter &
    \textbf{92.209$\pm$0.003}&
    91.152$\pm$0.003 ($<$\textbf{0.001}) &
    91.184$\pm$0.003 ($<$\textbf{0.001}, 0.484)&
    79.268$\pm$0.005 ($<$\textbf{0.001}, $<$\textbf{0.001})\\
    
    &
    ROI-1-CC&
    \textbf{92.386$\pm$0.003}&
    91.205$\pm$0.003 ($<$\textbf{0.001})&
    91.260$\pm$0.003 ($<$\textbf{0.001}, 0.009)&
    79.017$\pm$0.006 ($<$\textbf{0.001}, $<$\textbf{0.001})\\
    
    &
    ROI-2-MCP &
    \textbf{84.892$\pm$0.006}&
    82.907$\pm$0.007 ($<$\textbf{0.001})& 
    83.053$\pm$0.006 ($<$\textbf{0.001}, 0.032)& 
    68.396$\pm$0.009 ($<$\textbf{0.001}, $<$\textbf{0.001})\\
    
    &
    ROI-3-SLF &
    \textbf{93.290$\pm$0.003}& 
    92.372$\pm$0.003 (0.001)&
    92.375$\pm$0.003 ($<$\textbf{0.001}, $<$\textbf{0.001})&
    81.210$\pm$0.006 ($<$\textbf{0.001}, $<$\textbf{0.001})\\
    \specialrule{1.25pt}{0pt}{0pt}
    \multirow{4}{*}{\shortstack{\textbf{Fix}\\
    \textbf{Acc}\\
    (\uparrow)}} &
    White Matter &
    0.640$\pm$0.011& 
    \textbf{0.664$\pm$0.008} ($<$\textbf{0.001})&
    0.645$\pm$0.009 (0.037, $<$\textbf{0.001})&
    0.536$\pm$0.006 ($<$\textbf{0.001}, $<$\textbf{0.001})\\
    
    &
    ROI-1-CC&
    \textbf{0.901$\pm$0.002}& 
    0.851$\pm$0.005 ($<$\textbf{0.001})&
    0.867$\pm$0.003 ($<$\textbf{0.001}, 0.036)&
    0.469$\pm$0.010 ($<$\textbf{0.001}, $<$\textbf{0.001})\\
    
    &
    ROI-2-MCP &
    0.754$\pm$0.011& 
    \textbf{0.791$\pm$0.010} ($<$\textbf{0.001})&
    0.772$\pm$0.009 (0.001, 0.018)&
    0.548$\pm$0.009 ($<$\textbf{0.001}, $<$\textbf{0.001})\\
    
    &
    ROI-3-SLF &
    0.606$\pm$0.032& 
    \textbf{0.648$\pm$0.031} (0.001)&
    0.588$\pm$0.029 (0.023, $<$\textbf{0.001})&
    0.548$\pm$0.009 (0.076, 0.163)\\
    \specialrule{1.25pt}{0pt}{0pt}
    \multirow{4}{*}{\textbf{\shortstack{PAE \\  ($\downarrow$)}}} &
    White Matter &
    0.155$\pm$0.006& 
    \textbf{0.147$\pm$0.005} (\textbf{0.001})&
    0.152$\pm$0.005 (0.065, 0.011)&
    0.244$\pm$0.007 ($<$\textbf{0.001}, $<$\textbf{0.001})\\
    
    &
    ROI-1-CC&
    \textbf{0.062$\pm$0.002}& 
    0.072$\pm$0.002 ($<$\textbf{0.001})&
    0.069$\pm$0.002 (0.065, 0.011)&
    0.210$\pm$0.007 ($<$\textbf{0.001}, $<$\textbf{0.001})\\
    
    &
    ROI-2-MCP &
     \textbf{0.135$\pm$0.003}& 
     0.136$\pm$0.003 (0.393)&
     0.136$\pm$0.002 (0.065, 0.011)&
     0.219$\pm$0.004 ($<$\textbf{0.001}, $<$\textbf{0.001})\\
    &
    ROI-3-SLF &
     0.179$\pm$0.009& 
     \textbf{0.178$\pm$0.007} (0.779)&
     0.194$\pm$0.010 ($<$\textbf{0.001}, 0.053)&
     0.278$\pm$0.006 ($<$\textbf{0.001}, $<$\textbf{0.001})\\
    \specialrule{1.25pt}{0pt}{0pt}
    \multirow{4}{*}{\textbf{\shortstack{AFDE \\ (\downarrow)}}} &
    White Matter&
    0.164$\pm$0.005& 
    \textbf{0.151$\pm$0.004} ($<$\textbf{0.001})&
    0.160$\pm$0.005 (0.012, \textbf{0.002})&
    0.208$\pm$0.006 ($<$\textbf{0.001}, $<$\textbf{0.001})\\
    
    &
    ROI-1-CC&
    \textbf{0.065$\pm$0.001}& 
    0.074$\pm$0.001 ($<$\textbf{0.001})&
    0.073$\pm$0.002 (0.002, 0.711)&
    0.187$\pm$0.007 ($<$\textbf{0.001}, $<$\textbf{0.001})\\
    
    &
    ROI-2-MCP &
     0.107$\pm$0.002& 
     \textbf{0.105$\pm$0.001} (0.526)&
     0.106$\pm$0.001 (0.713, 0.489)&
     0.171$\pm$0.003 ($<$\textbf{0.001}, $<$\textbf{0.001})\\
    
    &
    ROI-3-SLF&
     0.151$\pm$0.007& 
     \textbf{0.149$\pm$0.006} (0.462)&
     0.165$\pm$0.007 ($<$\textbf{0.001}, $<$\textbf{0.001})&
     0.230$\pm$0.006 ($<$\textbf{0.001}, $<$\textbf{0.001})\\
    \specialrule{1.25pt}{0pt}{0pt}
  \end{tabular}}
  \caption{Quantitative results for all performance metrics, methods and regions of interest. $\text{p}_{SD}$ is the p-value for the paired t-test between the respective method and SDNet, $\text{p}_{SD \kappa}$ is the p-value for the paired t-test between the respective method and $\text{SDNet}_{\kappa}$.}
  \label{tab:QuantRes}
\end{table*}

 \begin{table*}
  \centering
  \resizebox{1\textwidth}{!}{
  \begin{tabular}{?l?l?llll?}
     \specialrule{1.25pt}{0pt}{0pt}
    \textbf{Metric} &\diagbox[innerwidth=2cm]{\textbf{Method}}{\textbf{Region}}& \textbf{White Matter} & \textbf{ROI-1-CC} & \textbf{ROI-2-MCP} & \textbf{ROI-3-SLF}\\
    \specialrule{1.1pt}{0pt}{0pt}
    \multirow{4}{*}{\textbf{SSE}} & 
    White Matter &
    0.011$\pm$0.001 &
    0.009$\pm$0.001 &
    0.020$\pm$0.001 & 
    0.012$\pm$0.001 \\
    \cline{2-6}
    &
    ${\text{SDNet}}_{\kappa}$ ($\text{p}_{\text{SD}}$)&
    0.012$\pm$0.001 ($$<$$\textbf{0.001}) &
    0.010$\pm$0.001 ($$<$$\textbf{0.001}) &
    0.022$\pm$0.001 ($$<$$\textbf{0.001}) &
    0.013$\pm$0.001 (\textbf{0.005}$) \\
    \cline{2-6}
    &
    FODNet ($\text{p}_{\text{SD}}, {\text{p}}_{\text{SD}\kappa}$) &
    0.013$\pm$0.001 $ {\textbf{($$<$$0.001}}, 0.034)$ &
    0.011$\pm$0.001 $ {\textbf{($$<$$0.001}}, 0.295)$&
    0.022$\pm$0.001 $ {\textbf{(0.001}}, 0.175)$ &
    0.014$\pm$0.001 $ {\textbf{($$<$$0.001}}, {\textbf{$$<$$0.001)}}$ \\
    \cline{2-6}
    &
    MSMT CSD ($\text{p}_{\text{SD}}, {\text{p}}_{\text{SD}\kappa}$) & 
    0.041$\pm$0.002 $ \textbf{($$<$$0.001}, \textbf{$$<$$0.001)}$ &
    0.037$\pm$0.002 $ \textbf{($$<$$0.001}, \textbf{$$<$$0.001)}$ & 
    0.057$\pm$0.003 $ \textbf{($$<$$0.001}, \textbf{$$<$$0.001)}$ & 
    0.043$\pm$0.002 $ \textbf{($$<$$0.001}, \textbf{$$<$$0.001)}$ \\
    \specialrule{1.25pt}{0pt}{0pt}
    \multirow{4}{*}{\textbf{ACC}} &
    SDNet &
    92.209$\pm$0.003 &
    92.386$\pm$0.003 &
    84.892$\pm$0.006 &
    93.290$\pm$0.003 \\
    \cline{2-6}
    &
    ${\text{SDNet}}_{\kappa}$ ($\text{p}_{\text{SD}}$)&
    91.152$\pm$0.003 $ \textbf{($$<$$0.001)}$&
    91.205$\pm$0.003  $\textbf{($$<$$0.001)}$ &
    82.907$\pm$0.007 $ \textbf{($$<$$0.001)}$ &
    92.372$\pm$0.003 $ \textbf{(0.001)}$ \\
    \cline{2-6}
    &
    FODNet ($\text{p}_{\text{SD}}$ (${\text{p}}_{\text{SD}\kappa}$) &
    91.184$\pm$0.003 ${\textbf{($$<$$0.001}}, 0.484)$&
    91.260$\pm$0.003 $ {\textbf{($$<$$0.001}}, 0.009)$ & 
    83.053$\pm$0.006 $ {\textbf{($$<$$0.001}}, 0.032)$ & 
    92.375$\pm$0.003 $ {\textbf{($$<$$0.001}}, {\textbf{$$<$$0.001)}}$\\
    \cline{2-6}
    &
    MSMT CSD ($\text{p}_{\text{SD}}, {\text{p}}_{\text{SD}\kappa}$) &
    79.268$\pm$0.005 $ \textbf{($$<$$0.001}, \textbf{$$<$$0.001)}$& 
    79.017$\pm$0.006 $ \textbf{($$<$$0.001}, \textbf{$$<$$0.001)}$ &
    68.396$\pm$0.009 $ \textbf{($$<$$0.001}, \textbf{$$<$$0.001)}$ &
    81.210$\pm$0.006 $ \textbf{($$<$$0.001}, \textbf{$$<$$0.001)}$ \\
    \specialrule{1.25pt}{0pt}{0pt}
    \multirow{4}{*}{\textbf{Fix Acc}} &
    SDNet &
    0.640$\pm$0.011& 
    0.901$\pm$0.002&
    0.754$\pm$0.011&
    0.606$\pm$0.032\\
    \cline{2-6}
    &
    ${\text{SDNet}}_{\kappa}$ ($\text{p}_{\text{SD}}$)&
    0.664$\pm$0.008 $ \textbf{($$<$$0.001)}$& 
    0.851$\pm$0.005 $\textbf{($$<$$0.001)}$&
    0.791$\pm$0.010 $ \textbf{($$<$$0.001)}$&
    0.648$\pm$0.031 $ \textbf{(0.001)}$\\
    \cline{2-6}
    &
    FODNet ($\text{p}_{\text{SD}}, {\text{p}}_{\text{SD}\kappa}$) &
    0.645$\pm$0.009 $ (0.037, \textbf{$$<$$0.001)}$& 
    0.867$\pm$0.003 $\textbf{($$<$$0.001}, 0.036)$&
    0.772$\pm$0.009 $\textbf{(0.001}, 0.018)$&
    0.588$\pm$0.029 $(0.023, \textbf{$$<$$0.001})$\\
    \cline{2-6}
    &
    MSMT CSD ($\text{p}_{\text{SD}}, {\text{p}}_{\text{SD}\kappa}$) &
    0.536$\pm$0.006 $\textbf{($$<$$0.001}, \textbf{$$<$$0.001})$& 
    0.469$\pm$0.010 $\textbf{($$<$$0.001}, \textbf{$$<$$0.001})$&
    0.548$\pm$0.009 $\textbf{($$<$$0.001}, \textbf{$$<$$0.001})$&
    0.548$\pm$0.009 $(0.076, 0.163)$\\
    \specialrule{1.25pt}{0pt}{0pt}
    \multirow{4}{*}{\textbf{PAE}} &
    SDNet &
    0.155$\pm$0.006 & 
    0.062$\pm$0.002&
    0.135$\pm$0.003&
    0.179$\pm$0.009\\
    \cline{2-6}
    &
    ${\text{SDNet}}_{\kappa} (\text{p}_{\text{SD}}$)&
    0.147$\pm$0.005 $ \textbf{(0.001)}$& 
    0.072$\pm$0.002 $ \textbf{($$<$$0.001)}$&
    0.136$\pm$0.003 $(0.393)$&
    0.178$\pm$0.007 $(0.779)$\\
    \cline{2-6}
    &
    FODNet ($\text{p}_{\text{SD}}, {\text{p}}_{\text{SD}\kappa}$) &
    0.152$\pm$0.005 $ \textbf{(0.065, 0.011)}$& 
    0.069$\pm$0.002 $\textbf{(0.065, 0.011)}$&
    0.136$\pm$0.002 $(0.065, 0.011)$&
    0.194$\pm$0.010 $ (\textbf{$$<$$0.001}, 0.053)$\\
    \cline{2-6}
    &
    MSMT CSD ($\text{p}_{\text{SD}}, {\text{p}}_{\text{SD}\kappa}$) &
    0.244$\pm$0.007 $\textbf{($$<$$0.001}, \textbf{$$<$$0.001)}$& 
    0.210$\pm$0.007 $\textbf{($$<$$0.001}, \textbf{$$<$$0.001)}$&
    0.219$\pm$0.004 $\textbf{($$<$$0.001}, \textbf{$$<$$0.001)}$&
    0.278$\pm$0.006 $\textbf{($$<$$0.001}, \textbf{$$<$$0.001)}$\\
    \specialrule{1.25pt}{0pt}{0pt}
    \multirow{4}{*}{\textbf{AFDE}} &
    SDNet&
    0.164$\pm$0.005& 
    0.065$\pm$0.001&
    0.107$\pm$0.002&
    0.151$\pm$0.007\\
    \cline{2-6}
    &
    ${\text{SDNet}}_{\kappa}$ ($\text{p}_{\text{SD}}$)&
     0.151$\pm$0.004 $ \textbf{($$<$$0.001)}$& 
     0.074$\pm$0.001 $ \textbf{($$<$$0.001)}$&
     0.105$\pm$0.001 $(0.526)$&
     0.149$\pm$0.006 $(0.462)$\\
    \cline{2-6}
    &
    FODNet ($\text{p}_{\text{SD}}, {\text{p}}_{\text{SD}\kappa}$) &
    0.160$\pm$0.005 $(0.012, \textbf{0.002)}$& 
    0.073$\pm$0.002 $ \textbf{(0.002}, 0.711)$&
    0.106$\pm$0.001 $ (0.713, 0.489)$&
    0.165$\pm$0.007 $ \textbf{($$<$$0.001}, \textbf{$$<$$0.001)}$\\
    \cline{2-6}
    &
    MSMT CSD (p_{\text{SD}}, {\text{p}}_{\text{SD}\kappa}) &
    0.208$\pm$0.006 $\textbf{($$<$$0.001}, \textbf{$$<$$0.001)}$& 
    0.187$\pm$0.007 $\textbf{($$<$$0.001}, \textbf{$$<$$0.001)}$&
    0.171$\pm$0.003 ($$<$$\textbf{0.001}, $$<$$\textbf{0.001})$&
    0.230$\pm$0.006 ($$<$$\textbf{0.001}, $$<$$\textbf{0.001})\\
    \specialrule{1.25pt}{0pt}{0pt}
  \end{tabular}}
  \caption{Quantitative results for all performance metrics, methods and regions of interest. $\text{p}_{SD}$ is the p-value for the paired t-test between the respective method and SDNet, $\text{p}_{SD \kappa}$ is the p-value for the paired t-test between the respective method and $\text{SDNet}_{\kappa}$.}
  \label{tab:QuantRes}
\end{table*}

\begin{table*}[ht]
\caption{Comparing different state-of-the-arts on 2D OASIS. The first, second, and third ranks are highlighted in  \textcolor{red}{red}, \textcolor{blue}{blue}, and \textcolor{brown}{brown} colors, respectively.}
\centering
\label{tab:oasis2d}
% \resizebox{\columnwidth}{!}{
\begin{small}
\begin{tabular}{lcccccccc}\hline
Methods     & Patch & Dice        & $|J|_{ < 0}\%$  & Parameters   & Mult-Adds (M) & Memory (MB)   & CPU (s) & GPU (s) \\\hline
Initial       & - & 0.544$\pm$0.089 &-           &-&-& - & -      \\
Flash       & 16$\times$16      & 0.702$\pm$0.051 & 0.033$\pm$.126  & - & - & - & 13.699 & - \\
Flash       & 20$\times$24      & 0.727$\pm$0.046 & 0.205$\pm$.279 & - & - & - &  22.575 & -    \\
Flash       & 40$\times$48      & 0.734$\pm$0.045 & 0.049$\pm$.080 & - & -& - & 85.773 & -    \\
DeepFlash   & 16$\times$16      & 0.615$\pm$0.055 & 0.0$\pm$0.0            & - & - & -& 0.487      &-   \\
DeepFlash   & 20$\times$24      & 0.597$\pm$0.066            & 0.0$\pm$0.0 & - & - & -&0.617    &-     \\
% DeepFlash   & 40x48      &             &             &     &     \\
B-Spline-Diff   & 20$\times$24      & 0.710$\pm$0.041 &  0.014$\pm$0.072 & 70,226 & 86.16 & 6.58   &0.012     &0.015     \\
B-Spline-Diff   & 40$\times$48      & 0.737$\pm$0.038  & 0.015$\pm$0.069 & 88,690    & 139.40 & 7.49    &0.012 &0.015 \\\hline
Fourier-Net$_{\text{Small}}$ &40$\times$48     & 0.748$\pm$0.039  & 0.672$\pm$0.391   &357,408          & 224.55 & 17.96    & \textbf{0.007}     & \textbf{0.014} \\
Fourier-Net-Diff$_{\text{Small}}$ &40$\times$48     & 0.750$\pm$0.038  & $<$0.0001         &357,408    & 224.55 & 17.96    & 0.010     & 0.014 \\  
Fourier-Net &40$\times$48     & 0.756$\pm$0.039  & 0.753$\pm$0.408       &1,427,376     & 888.25 & 35.89     & 0.011     & 0.015    \\
Fourier-Net-Diff &  40$\times$48 & 0.756$\pm$0.037  & $<$0.0001 &1,427,376 & 888.25 & 35.89  & 0.015     & 0.015   \\
% Fourier-Net${_{Large}}$ &40$\times$48     & 0.759$\pm$0.040  & 0.781$\pm$0.405             & 0.131     & 0.023    \\
% Fourier-Net-Diff${_{Large}}$ &  40$\times$48 & \textbf{0.761$\pm$0.037}  & 0.0$\pm$0.0   & 0.040     & 0.024   \\\hline
1$\times$Fourier-Net++       & 40$\times$48   & 0.738$\pm$0.041  & 0.674$\pm$0.377 &300,477 & 142.66         & 9.52 & 0.006 & 0.014\\
1$\times$Fourier-Net++-Diff  & 40$\times$48   & 0.740$\pm$0.039  & 0.0$\pm$0.0    &300,477 & 142.66         & 9.52 & 0.009 & 0.014\\
4$\times$Fourier-Net++$_{\text{Small}}$ &  40$\times$48 & 0.757$\pm$0.039  & 0.252$\pm$0.197 &301,716 & 145.44         & 19.12 & 0.018 & 0.017\\
4$\times$Fourier-Net++-Diff$_{\text{Small}}$ &  40$\times$48 &0.746$\pm$0.040  & 0.0$\pm$0.0      &301,716 & 145.44         & 19.12 & 0.021 & 0.017\\
4$\times$Fourier-Net++ &  40$\times$48 & 0.761$\pm$0.039  & 0.278$\pm$0.232 &1,201,908 & 570.64        & 38.08 & 0.022 & 0.017\\
4$\times$Fourier-Net++-Diff &  40$\times$48 &0.755$\pm$0.039  & $<$0.0001     &1,201,908  & 570.64         & 38.08 & 0.025 & 0.017\\\hline
\end{tabular}
\end{small}
% }
\end{table*}
